# Supplementary material for: AutoCode: LLMs as Problem Setters for Competitive Programming
Source: arXiv:2510.12803 source file (2025-09-29)
Supplement: Supplementary file 1 [file 6_related_work.tex]

\section{Additional Related Works}
\label{appendix:related_works}

In this section, we expand the discussion of related works by providing more detailed descriptions of highly related relevant works, including CodeContests~\cite{li2022competition}, TACO~\cite{li2023taco}, CodeContests+~\cite{wang2025codecontests+}, HardTests~\cite{he2025hardtests}, TestCase-Eval~\cite{cao2025can}, and LogiCase~\cite{sung2025logicase}, and connect our work to the growing body of literature on self-play and self-improvement. 

\paragraph{CodeContests~\cite{li2022competition}.} CodeContests is a large-scale competitive programming dataset originally compiled to train and evaluate DeepMind's AlphaCode model. It contains thousands of coding problems from platforms such as Codeforces, CodeChef, and others, each paired with a set fo input-output test cases and a collection of submitted solutions (both correct and incorrect). The test suites were partly generated through simple rule-based mutations of known examples and validated through known correct solutions. In particular, each mutated input was validated by running 30 known correct human solutions and keeping it only if all 30 produced the same output. Note that our work explicitly avoid using existing known solutions of constructed problems because we aim at automatically generating novel problems which don't have known correct solutions to begin with.

\paragraph{TACO~\cite{li2023taco}.} TACO (Topics in Algorithmic COde generation) is an open-source benchmark dataset of over 26000 competition-level questions, accompanied by a set of 1.55 million solution attempts. Each problem is annotated with fine-grained metadata such as topics, algorithms, required skills, and difficulty level.

\paragraph{CodeContests+~\cite{wang2025codecontests+}.} CodeContests+ was introduced to improve upon CodeContests by generating higher-quality test cases using an LLM-based generator-validator agent framework. CodeContests+ increased evaluation accuracy over CodeContests and doesn't depend on existing known solutions to check the validity of the generated test cases.

\paragraph{HardTests~\cite{he2025hardtests}.} HardTests similarly targets tricky edge-case tests for code evaluation, but at an even larger scale. It introduces a pipeline called HARDTESTGEN that leverages LLMs to generate and filter test cases for competitive programming tasks. Using this pipeline, the authors constructed a HARDTESTS dataset spanning 47000 problems. The generated test cases are specifically designed to uncover subtly incorrect solutions that fail under extreme conditions.

\paragraph{TestCase-Eval~\cite{cao2025can}.} TestCase-Eval is a benchmark specifically designed to assess how well LLMs can produce test cases for algorithmic problems. It compiles 500 coding problems (drawn from Codeforces and similar contests) along with 100,000 human-written solutions, including many that are incorrect in know ways. The benchmark defines two core metrics: {\em Fault coverage}, measuring how well LLM-generated test sets cover a wide range of failure modes, and {\em fault exposure}, which evaluates whether LLMs can craft targeted inputs that cause a specific flawed solution to fail. In experiments with 19 state-of-the-art LLMs, TestCase-Eval revealed varying strengths and limitations in their test generation abilities: for example, some models excel at generating diverse inputs but struggle to pinpoint particular edge-case failures, and vice versa.

\paragraph{LogiCase~\cite{sung2025logicase}.} LogiCase introduces and approach that combines learning with logical specification to generate test cases. In particular, LogiCase uses a neural model to translate the problem's natural language input description (e.g., the formal specification of input format and constraints) into a machine-interpretable grammar. Specifically, it introduces Context-Free Grammars with Counters (CCFGs), a formalism that captures both syntactic and semantic structures in input specifications. From this grammar, LogiCase then automatically enumerates valid test cases, enabling systematic generation of test cases.

Our work, on the other hand, not only achieves state-of-the-art test case generation quality, but also automates the entire problem generation process by leveraging seed problems and cross-verification with brute-force solutions. This fully automated process opens the possibility for model self-play and self-improvement. In parallel, there is a growing body of literature studying how models can improve using their own signals: STaR~\cite{zelikman2022starbootstrappingreasoningreasoning} bootstraps reasoning by generating rationales and fine-tuning on those that yield correct answers. Quiet-STaR~\cite{zelikman2024quietstarlanguagemodelsteach} extended this idea to token-level rationales in general text, enabling broader self-supervision. Iterative self-correction paradigms such as Reflexion~\cite{shinn2023reflexionlanguageagentsverbal} and Self-Refine~\cite{madaan2023selfrefineiterativerefinementselffeedback} further demonstrate gains across coding and reasoning tasks. SPC (Self-Play Critic)~\cite{chen2025spcevolvingselfplaycritic} evolves a process-level judge through adversarial games between a step generator and a critic, improving chain-of-thought evaluation without step-level human labels. SeRL (Self-Play Reinforcement Learning)~\cite{fang2025serlselfplayreinforcementlearning} bootstraps training with limited data by letting a model act as both opponent and teach under self-play reinforcement learning. SPIRAL~\cite{liu2025spiralselfplayzerosumgames} shows that self-play on zero-sum games incentivizes reasoning via multi-agent multi-turn reinforcement learning. RLSF (Reinforcement Learning from Self-Feedback)~\cite{vanniekerk2025posttraininglargelanguagemodels} uses the model's own confidence as an intrinsic reward. SEAL (Self-Adapting LLMs)~\cite{zweiger2025selfadaptinglanguagemodels} enables LLMs to self-adapt by generating their own finetuning data and update directives. Our framework, AutoCode, significantly advances this line of effort by coupling high-quality and diverse problem design using the idea of seed problems with state-of-the-art test case generation, providing a ready-made environment for highly-capable models to self-train and self-evolve.
