# Supplementary material for: AutoCode: LLMs as Problem Setters for Competitive Programming
Source: arXiv:2510.12803 source file (2025-09-29)
Supplement: Supplementary file 2 [file 7_ethics.tex]

\section*{Ethics Statement}
\label{appendix:ethics}

This study adheres to the ethical standards of academic research. The benchmark datasets we used are all publicly available from competitive programming platforms (such as Codeforces and AtCoder), and do not involve any personal privacy data or sensitive information. All data were filtered and anonymized, and used solely for algorithm evaluation and model validation. Furthermore, the experiments did not cause any direct or indirect harm to individuals or groups. We recognize that automated problem generation may be misused, for example in cheating or spreading low-quality content. Therefore, we emphasize the critical role of human experts in the final screening and evaluation. We advocate for the responsible and reasonable use of the outcomes of this research.
