# Supplementary material for: AutoCode: LLMs as Problem Setters for Competitive Programming
Source: arXiv:2510.12803 source file (2025-09-29)
Supplement: Supplementary file 3 [file 8_reproduce.tex]

\section*{Reproducibility Statement}
\label{appendix:reproduce}

To ensure reproducibility, we provide a complete description of the framework design, including the construction of the Validator, Generator, Checker, and Interactor (see Section 2 of the main text). Algorithm pseudocode and process diagrams are detailed in the appendix, along with concrete steps for validation data construction, problem generation, and the dual-verification protocol. All experiments were conducted on publicly available benchmarks (CodeContests+, TACO, HardTests, etc.) as well as on recent Codeforces problems. We report ablation studies (Table~\ref{tab:ablation}) and comparisons with existing methods (Table~\ref{tab:main_results}), supplemented with statistical significance analysis.
