# Supplementary material for: AutoCode: LLMs as Problem Setters for Competitive Programming
Source: arXiv:2510.12803 source file (2025-09-29)
Supplement: Supplementary file 4 [file 9_llm_usage.tex]

\section*{The use of Large Language Models}
\label{appendix:llm}

The main contributions of this work rely on the generative and discriminative capabilities of LLMs. Specifically, LLMs are employed in a multi-role framework as generator, validator, and checker. During training and experimentation, we use publicly accessible LLM APIs (\eg\texttt{GPT-5-High}) without additional fine-tuning. It is important to note that while LLMs can automatically generate new problems, the quality and novelty of these problems still require expert evaluation and filtering. We firmly believe LLMs should serve as auxiliary tools to expand data generation and test coverage, rather than as replacements for human creative judgment. In addition, LLMs are partially used during the writing stage of this paper for language polishing and improving clarity of expression.
